# Supplementary material for: Microtopia: Exploring the Impact of Interdisciplinary Projects on Ethnic Minority Female Pupils' Perceptions of Computer Science
Source: arXiv:2512.21214 source file (2025-12-24)
Supplement: Supplementary file 1 [file Appendix-RQ3WilcoxonSignedRankTest.tex]

\section{Microtopia’s Influence on Pupils’ Perceptions of Computer Science}
\label{appendix:WilcoxonEthnicity}
\begin{table}[h!]
\centering
\small
\caption{Pre- and Post-test results with Wilcoxon Signed Rank Test (Mean (M), SD, SE, Z, p).}
\label{tab:CSWilcoxonSignedTestAll}
\resizebox{\textwidth}{!}{%
\begin{tabular}{p{7cm}ccccc}
\hline
\textbf{Statement} & \textbf{Pre-test M (SD, SE)} & \textbf{Post-test M (SD, SE)} & \textbf{Z} & \textbf{p} \\
\hline
\multicolumn{5}{l}{\textbf{CS Perceptions}} \\
I feel confident in my skills when using a computer. & $3.47 \,(1.02,\,0.11)$ & $4.23 \,(0.84,\,0.09)$ & $-7.39$ & $p < .001$ \\
I believe computer science is enjoyable. & $3.18 \,(1.17,\,0.12)$ & $3.99 \,(0.98,\,0.10)$ & $-7.39$ & $p < .001$ \\
I am interested in studying computer science. & $3.09 \,(1.24,\,0.13)$ & $3.82 \,(1.07,\,0.11)$ & $-7.17$ & $p < .001$ \\
I feel good about learning/studying computer science. & $3.44 \,(1.10,\,0.12)$ & $3.78 \,(0.97,\,0.10)$ & $-6.22$ & $p = .010$ \\
I am confident in my ability to do well in computer science courses. & $3.32 \,(1.05,\,0.11)$ & $3.81 \,(1.04,\,0.11)$ & $-7.44$ & $p < .001$ \\
I think computer science is for boys only. & $1.19 \,(0.47,\,0.05)$ & $1.28 \,(0.90,\,0.09)$ & $-7.84$ & $p = .540$ \\
I think that boys and girls can be good at computer science. & $4.72 \,(0.64,\,0.07)$ & $4.79 \,(0.53,\,0.06)$ & $-7.77$ & $p = .467$ \\
I want to have a job someday that involves computers. & $3.20 \,(1.17,\,0.12)$ & $3.39 \,(1.22,\,0.13)$ & $-6.56$ & $p = .038$ \\
I believe anyone can learn computer science. & $4.52 \,(0.72,\,0.08)$ & $4.30 \,(0.92,\,0.10)$ & $-7.39$ & $p = .042$ \\
I believe that learning computer science is hard. & $3.42 \,(1.02,\,0.11)$ & $2.74 \,(1.14,\,0.12)$ & $-6.75$ & $p < .001$ \\
People who do computer science need to be very smart. & $3.30 \,(1.10,\,0.12)$ & $3.01 \,(1.14,\,0.12)$ & $-6.07$ & $p = .047$ \\
\hline
\multicolumn{5}{l}{\textbf{Collaboration \& Teamwork}} \\
I feel good about working with my teammates on projects. & $3.92 \,(0.99,\,0.10)$ & $4.33 \,(0.95,\,0.10)$ & $-7.04$ & $p < .001$ \\
I think it is important for us to work together when we have tasks to do. & $4.23 \,(0.82,\,0.09)$ & $4.34 \,(0.90,\,0.10)$ & $-6.95$ & $p = .194$ \\
I like when we all help each other to finish our work. & $4.26 \,(0.92,\,0.10)$ & $4.39 \,(0.96,\,0.10)$ & $-6.73$ & $p = .139$ \\
It’s easy for me to talk to my teammates and share my ideas when we’re working on something. & $3.96 \,(1.07,\,0.11)$ & $4.36 \,(0.93,\,0.10)$ & $-7.31$ & $p < .001$ \\
I am okay with doing different jobs in our group when we need to. & $4.14 \,(0.79,\,0.08)$ & $4.34 \,(0.81,\,0.09)$ & $-6.64$ & $p = .036$ \\
I think it’s cool when we have all sorts of different people in our group. & $4.21 \,(1.07,\,0.11)$ & $4.40 \,(0.82,\,0.09)$ & $-7.47$ & $p = .095$ \\
I would not mind being the only girl in a group. & $3.46 \,(1.81,\,0.19)$ & $2.51 \,(1.44,\,0.15)$ & $-5.40$ & $p = .001$ \\
I do not think I can work well if I am the only girl in a group. & $2.42 \,(1.41,\,0.15)$ & $1.27 \,(0.85,\,0.09)$ & $-7.28$ & $p < .001$ \\
I do not think I work well in a group. & $1.76 \,(0.98,\,0.10)$ & $1.93 \,(1.22,\,0.13)$ & $-6.43$ & $p = .216$ \\
\hline
\multicolumn{5}{l}{\textbf{Interdisciplinary}} \\
I think that computer science requires different subjects and fields, like science, art, physics, design, social sciences, or maths. & $4.00 \,(0.91,\,0.10)$ & $4.24 \,(0.94,\,0.10)$ & $-6.23$ & $p = .028$ \\
I think that computer science is used in different subjects and fields, like science, art, physics, design, social sciences, or maths. & $4.16 \,(0.94,\,0.10)$ & $4.32 \,(0.76,\,0.08)$ & $-6.69$ & $p = .117$ \\
\hline
\multicolumn{5}{l}{\textbf{Future in CS}} \\
I want to learn more about computer science in the future & $3.99 \,(0.93,\,0.10)$ & $4.29 \,(0.80,\,0.08)$ & $-6.45$ & $p = .011$ \\
I want to study computer science at university & $2.57 \,(1.02,\,0.11)$ & $2.86 \,(1.37,\,0.14)$ & $-5.18$ & $p = .080$ \\
I want a job in the future that uses computer science & $4.26 \,(0.73,\,0.08)$ & $4.21 \,(1.03,\,0.11)$ & $-6.67$ & $p = 1.000$ \\
I think I can be successful in computer science if I work hard & $3.73 \,(1.01,\,0.11)$ & $4.21 \,(0.85,\,0.09)$ & $-7.45$ & $p < .001$ \\
\hline
\end{tabular}%
}
\end{table}
\subsection{Asian Ethnic Pupils’ Perceptions of Computer Science} 
Asian students showed the broadest pattern of significant improvements across all sections. Attitudinally, they reported higher confidence, enjoyment, and interest in computer science after the workshop, and stronger beliefs in their own ability to succeed. Importantly, negative perceptions — such as “CS is hard” and “CS is only for very smart people” — decreased significantly. In terms of collaboration, Asian students became more comfortable sharing ideas, working in diverse groups, and reported reduced discomfort with being the only girl in a group. They also shifted away from preferring to work alone. Additionally, Asian students recognised more strongly that computer science requires multiple disciplines, expressed greater aspirations to continue learning CS, and more strongly believed that CS can help address global challenges. Overall, this group exhibited the most consistent and wide-ranging positive changes.
\begin{table}[h!]
\centering
\small
\caption{Significant Pre- and Post-test results with Wilcoxon Signed Rank Test for Asian students.}
\label{tab:CSWilcoxonSignedTest_Asian}
\resizebox{\textwidth}{!}{%
\begin{tabular}{p{7cm}ccccc}
\hline
\textbf{Statement} & \textbf{Pre-test M (SD, SE)} & \textbf{Post-test M (SD, SE)} & \textbf{Z} & \textbf{p} \\
\hline
\multicolumn{5}{l}{\textbf{CS Perceptions}} \\
I feel confident in my skills when using a computer. & 3.41 (1.00, 0.12) & 4.37 (0.98, 0.12) & -5.82 & $p<.001$ \\
I believe computer science is enjoyable. & 3.21 (1.15, 0.14) & 4.43 (0.87, 0.11) & -6.30 & $p<.001$ \\
I am interested in studying computer science. & 3.04 (1.23, 0.15) & 4.50 (0.91, 0.11) & -6.42 & $p<.001$ \\
I feel good about learning/studying computer science. & 3.49 (1.11, 0.13) & 4.44 (0.90, 0.11) & -5.60 & $p<.001$ \\
I am confident in my ability to do well in computer science courses. & 3.32 (1.09, 0.13) & 4.37 (0.83, 0.10) & -6.53 & $p<.001$ \\
I believe that learning computer science is hard. & 3.50 (0.97, 0.12) & 1.65 (1.22, 0.15) & -6.61 & $p<.001$ \\
People who do computer science need to be very smart. & 3.35 (1.03, 0.13) & 1.84 (1.19, 0.14) & -6.49 & $p<.001$ \\
\hline
\multicolumn{5}{l}{\textbf{Collaboration \& Teamwork}} \\
It’s easy for me to talk to my teammates and share my
ideas when we’re working on something.& 4.07 (1.07, 0.13) & 4.44 (0.90, 0.11) & -6.50 & 0.003 \\
I think boys and girls can work together well in a group. & 4.35 (0.86, 0.10) & 3.50 (1.58, 0.19) & -6.61 & $p<.001$ \\
I do not think I can work well if I am the only girl in a group. & 2.43 (1.45, 0.18) & 1.22 (0.81, 0.10) & -6.60 & $p<.001$ \\
I think that a computer science club is a boy’s club. & 1.26 (0.66, 0.08) & 1.65 (1.22, 0.15) & -6.59 & 0.038 \\
I like working alone than working in a team. & 2.38 (1.29, 0.16) & 4.29 (1.12, 0.14) & -6.41 & $p<.001$ \\
\hline
\multicolumn{5}{l}{\textbf{Interdisciplinary}} \\
CS requires different subjects and fields. & 4.06 (0.91, 0.11) & 4.32 (0.92, 0.11) & -5.42 & 0.049 \\
\hline
\multicolumn{5}{l}{\textbf{Future in CS}} \\
I want to learn more about computer science in the future. & 4.09 (0.86, 0.10) & 4.40 (0.76, 0.09) & -5.73 & 0.022 \\
I think I can be successful in computer science if I work hard. & 3.74 (1.07, 0.13) & 4.32 (0.80, 0.10) & -6.72 & $p<.001$ \\
\hline
\end{tabular}%
}
\end{table}
\subsection{Black Ethnic Pupils’ Perceptions of Computer Science} 
Black students demonstrated a smaller but still meaningful set of significant changes. In Section 3, they showed increased interest in studying CS and improved perceptions of learning CS as enjoyable, alongside reduced agreement that “CS is hard”. In collaboration, they expressed less agreement with the idea that they cannot work well if the only girl in a group, suggesting a gain in confidence about inclusive teamwork. In aspirations, they also expressed a stronger desire to learn more about CS in the future. Taken together, these results suggest that while the breadth of change was narrower than for Asian students, Black students benefitted particularly in terms of interest, perceived difficulty, and willingness to pursue further CS learning.
\begin{table}[h!]
\centering
\small
\caption{Significant Pre- and Post-test results with Wilcoxon Signed Rank Test for Black students.}
\label{tab:CSWilcoxonSignedTest_Black}
\resizebox{\textwidth}{!}{%
\begin{tabular}{p{7cm}ccccc}
\hline
\textbf{Statement} & \textbf{Pre-test M (SD, SE)} & \textbf{Post-test M (SD, SE)} & \textbf{Z} & \textbf{p} \\
\hline
\multicolumn{5}{l}{\textbf{CS Perceptions}} \\
I am interested in studying computer science. & 3.33 (0.82, 0.33) & 4.33 (0.82, 0.33) & -2.20 & 0.034 \\
I feel good about learning/studying computer science. & 3.33 (0.52, 0.21) & 4.00 (0.63, 0.26) & -2.20 & 0.046 \\
I believe that learning computer science is hard. & 3.00 (1.26, 0.52) & 1.50 (0.84, 0.34) & -2.20 & 0.031 \\
\hline
\multicolumn{5}{l}{\textbf{Collaboration \& Teamwork}} \\
I do not think I can work well if I am the only girl in a group. & 3.17 (1.33, 0.54) & 1.00 (0.00, 0.00) & -2.20 & 0.031 \\
\hline
\multicolumn{5}{l}{\textbf{Future in CS}} \\
I want to learn more about computer science in the future. & 3.00 (0.89, 0.37) & 4.33 (0.52, 0.21) & -2.20 & 0.039 \\
\hline
\end{tabular}%
}
\end{table}
